# Supplementary material for: Analytic Performance Model of a Main-Memory Index Structure
Source: arXiv:1609.01319 source file (2017-04-05)
Supplement: Supplementary file 1 [file 60_appendix.tex]

\chapter{Appendix}

\section{First Appendix Section}
\label{sec:appendix:FirstSection}

\setcounter{figure}{0}

\begin{figure} [ht]
  \centering
  \missingfigure{A figure}
  \caption{A figure}
  \label{fig:anotherfigure}
\end{figure}
